# Supplementary material for: Grounded Video Situation Recognition
Source: arXiv:2210.10828 source file (2022-10-19)
Supplement: Supplementary file 1 [file 7_appendix.tex]

\section{Appendix}

Optionally include extra information (complete proofs, additional experiments and plots) in the appendix.
This section will often be part of the supplemental material.
